# Supplementary material for: Siamese Learning with Joint Alignment and Regression for Weakly-Supervised Video Paragraph Grounding
Source: arXiv:2403.11463 source file (2024-05-14)
Supplement: Supplementary file 1 [file X_suppl.tex]

\clearpage
\appendix
\setcounter{page}{1}
\setcounter{section}{0}
\setcounter{equation}{0}

\maketitlesupplementary

\section{Implementation Details}
In this supplementary material, we aim to provide more details about the two data augmentation strategies and the concrete formulations of the three auxiliary losses.
\subsection{Data Augmentation}
\noindent\textbf{Random Boundary Shifting (RBS).} To combat the potential synthesis artifacts and boundary uncertainty, the pseudo temporal labels in the augmentation branch are added with small random offsets for training. Concretely, the boundary offsets $\Delta I^{\text{st}}$ and $\Delta I^{\text{ed}}$ are randomly sampled from a uniform distribution ranging from 0 to the value of multiplying a percentage $p$ with the re-scaled length of the foreground video feature sequence. As a scalar hyper-parameter, the value of $p$ is 0.1, 0.175 and 0.1 for ActivityNet-Captions, Charades-CD-OOD and TACoS datasets, respectively.

\noindent\textbf{Random Re-Sampling (RRS).} We randomly re-scale the length of the foreground video to increase the sample diversity when generating the pseudo videos for training. The re-scaled feature sequence is obtained by a strided sampling operation from the original feature sequence. The stride is randomly acquired from a uniform distribution with a range of [0.75, 3], [1, 3] and [1, 15] for ActivityNet-Captions, Charades-CD-OOD and TACoS datasets, respectively.

\subsection{Auxiliary Losses}
\noindent\textbf{Cross-Branch Loss.} In our siamese learning framework, the augmentation branch and inference branch are designed for grounding the paragraph queries and sentence queries from different input video streams. The cross-branch loss $\mathcal{L}_\text{cb}$ aims to mine the potential supervision provided by the semantic consistent constraint as follows: 
\begin{equation}
    \begin{split}
    \mathcal{L}_{\text{cb}} = 1 - \text{Sim}\left(\mathcal{Q}_\text{aug}^\text{s}, \text{StopGrad}\left(\mathcal{Q}_\text{inf}^\text{s}\right)\right) + \\ 
    1 - \text{Sim}\left(\text{StopGrad}\left(\mathcal{Q}_\text{aug}^\text{p}\right), \mathcal{Q}_\text{inf}^\text{p}\right)
    \end{split}
\end{equation}
where $\mathcal{Q}_\text{aug}^\text{s}$ and $\mathcal{Q}_\text{inf}^\text{s}$ are the hidden features for sentence queries in decoder layers of the augmentation branch and the inference branch, respectively. Likewise, $\mathcal{Q}_\text{aug}^\text{p}$ and $\mathcal{Q}_\text{inf}^\text{p}$ are the hidden features for paragraph queries in the decoder layers of the augmentation branch and the inference branch, respectively. $\text{Sim}\left(\cdot\right)$ is the cosine similarity function and $\text{StopGrad}\left(\cdot\right)$ is the gradient-stopping operation.

\noindent\textbf{Anchor Ranking Loss.} As illustrated in the manuscript, there exists a chronological relationship between sentences in the same paragraph. Since our query decoder adopts a set of dynamic anchors to represent query-specific location information during the decoding process, the anchor ranking loss $\mathcal{L}_\text{ar}$ is employed to guide the intermediate query locations to be temporally ordered, which is given as follows: 
\begin{equation}
    \mathcal{L}_\text{ar} = \text{max}\left(0, d + \mathcal{C}\left(\mathcal{A}_\text{i}\right) - \mathcal{C}\left(\mathcal{A}_\text{i+1}\right)\right)
\end{equation}
where $\mathcal{A}_{i}$ and $\mathcal{A}_{i+1}$ are the anchor boxes of the $i$-th and $(i+1)$-th sentence queries of the last decoder layer in the inference branch, respectively. $\mathcal{C}\left(\cdot\right)$ denotes calculating the temporal center point of a given anchor box and $d$ is the distance that is set to $\frac{1}{2N}$, where $N$ is the number of sentences.

\noindent\textbf{Pseudo Attention Loss.} The ability of the query decoder in associating relevant visual content and textual descriptions can be directly reflected by the cross-modal attention weights produced by the query decoder layers. Based on the pseudo boundaries in the augmentation branch, we employ a loss to encourage the paragraph-to-video attention to be activated only within the relevant temporal regions. Specifically, we define the pseudo attention loss $\mathcal{L}_{\text{pa}}$ as:
\begin{equation}
    \mathcal{L}_{\text{pa}} = -\frac{1}{K_\text{dec}}\sum_{i=1}^{K_\text{dec}}\log\left(\sum_{t=1}^{T}m(t)\alpha_{\text{p}}^{(i)}(t)\right)
\end{equation}
where $\alpha_{\text{p}}^{(i)}(t)$ is the attention between the paragraph query and the $t$-th encoded clip feature at the 
$i$-th decoder layer. $m(t)$ denotes a mask that takes 1 for $t\in \left[\tau_{\text{aug}}^{\text{st}}, \tau_{\text{aug}}^{\text{ed}}\right]$ and takes 0 otherwise. $K_\text{dec}$ is the number of decoder layers.
